# Supplementary material for: Flexible Marginal Models for Dependent Data
Source: arXiv:2204.07188 source file (2022-04-14)
Supplement: Supplementary file 1 [file 07-appendix.tex]

%!TEX root = ../MMM_draft.tex

\section{A: Estimation}
\label{s:appendixA}
Estimation proceeds as follows:
\begin{enumerate}
	\item[~~~~\textbf{Step 1: }] Fit the conditional model (\ref{eqn:flexCond}).
	\item[~~~~\textbf{Step 2: }]  Use estimates and predictions  from the fitted conditional model in Step 1 to compute estimates of $\margmeanlinki_{ij}=\link\left\lbrace \margmeani_{ij}(\covx_{in_i})\right\rbrace$.
	\item[~~~~\textbf{Step 3: }]  Use the estimates $\margmeanlinkesti_{ij}$ from Step 2 as pseudo-outcomes, and fit the (marginal) additive model (\ref{eqn:flexMarg}).
\end{enumerate}
In practice, we can replace step 2 with a more general step to estimate  ${\lambda}_{*}^M=g({\mu}_{*}^M)$ for an arbitrary grid of covariate vectors, $\mathbf{x}_*$, but we use the observed data to simplify notation.

\subsection{Step 1: Fit the conditional model}
\label{ss:step1}
For simplicity, assume we have a single fixed effect covariate $\covxi_{ij}$, and write the conditional model
 \begin{align}
	\link\{\condmeani_{ij}(\covxi_{ij})\}&=\smoothfunC(\covxi_{ij})+ \covz_{ij}\tpose \re_{i}, \text{ ~~~ } \re_{i} \sim N(\mathbf{0},\boldsymbol{\Sigma})\label{eqn:flexCond1}
\end{align}
where $\condmeani_{ij}(\covxi_{ij})\equiv \EE(\datai_{ij}|\covxi_{ij},\covz_{ij},\re_{i})$. For some basis  $\{\condbasisfun_q(x)\}_{q=1}^Q$, we express
$\smoothfunC(x)=\sum_{q=1}^Q \condbasisfun_q (x) \condbasiscoefi_q$ with a quadratic penalty $\penaltyC{\condbasiscoef}\tpose \condSmat \condbasiscoef/2$ where $\condbasiscoef=[\condbasiscoefi_1,\dots,\condbasiscoefi_Q]^T$, $\condSmat$ is a known $Q\times Q$ positive semi definite matrix determined by the basis and $\penaltyC$ is a smoothing parameter to be estimated.  Write $\smoothfunC(\mathbf{x})=\condXbasis \condbasiscoef$ where $\condXbasis$ is the induced $\left(\sum_{i=1}^{\numclusters}\numunits_{i}\right)\times Q$ model matrix. Following \cite{wood2017generalized}, take the  eigendecomposition $\condSmat=\mathbf{U}\mathbf{D}\mathbf{U}\tpose$ where $\mathbf{U}$ is an orthonormal matrix of eigenvectors and $\mathbf{D}$ a diagonal matrix of decreasing non-negative eigenvalues. Let $[{\condbr}\tpose, {\condbetaF}\tpose]\tpose \equiv \mathbf{U}\tpose \condbasiscoef$, where $\condbetaF$ is of length $M$ and $\condbr$ is of length $Q-M$. Then it is easy to see that:
\begin{align*}
{\condbasiscoef}\tpose \condSmat \condbasiscoef&= {\condbasiscoef}\tpose \mathbf{U}\mathbf{D}\mathbf{U}\tpose \condbasiscoef \\
&={(\mathbf{U}\tpose \condbasiscoef)}\tpose \mathbf{D}(\mathbf{U}\tpose \condbasiscoef) \\
&=[{\condbr}\tpose, {\condbetaF}\tpose]\mathbf{D} [{\condbr}\tpose, {\condbetaF}\tpose]\tpose \\
&= {\condbr}\tpose \mathbf{D} _{+} {\condbr}
\end{align*}
where $\mathbf{D} _{+} $ is the $\left(Q-M\right)\times \left(Q-M\right)$ submatrix of $\mathbf{D}$ containing all positive eigenvalues. Hence only $\condbr$ is being penalized, not $\condbetaF$. As such we decompose $\mathbf{U}=[\UR,\UF]$ where $\UR$ has $Q-M$ columns and $\UF$ has $M$ columns, and let $\condXbasisR=\condXbasis \UR$ and $\condXbasisF=\condXbasis \UF$. Now we can re-express:
\begin{align*}
\smoothfunC(\mathbf{X})&=\condXbasis \condbasiscoef \\
&=\condXbasis \mathbf{U} \mathbf{U}\tpose \condbasiscoef \\
&=(\condXbasis \mathbf{U}) (\mathbf{U}\tpose \condbasiscoef )\\
&=\condXbasis [\UR,\UF] [{\condbr}\tpose, {\condbetaF}\tpose]\tpose \\
%&=\condXbasisF\condbetaF+ \condXbasisR\condbr \text{~~ where ~~} \condbr\sim N(\mathbf{0},[{\penaltyC}]^{-1}\mathbf{D}_{+}^{-1}).
&=\condXbasisF\condbetaF+ \condXbasisR\condbr \text{~~ subject to penalty ~~} \frac{1}{2}{\penaltyC} {\condbr}\tpose \mathbf{D}_{+} \condbr.
\end{align*}
Moreover, since $\boldsymbol{D}_{+}$ is known we can rewrite this as:
\begin{align*}
%\smoothfunC(\mathbf{X})&=\condXbasisF\condbetaF+ \condZbasisR\condbrscale  \text{~~ where ~~} \condbrscale \sim N(\mathbf{0},{\penaltyC}^{-1}\mathbf{I})  \text{~and~} \condZbasisR=\condXbasisR \boldsymbol{D}_{+}^{1/2}
\smoothfunC(\mathbf{X})&=\condXbasisF\condbetaF+ \condZbasisR\condbrscale  \text{~~ subject to penalty~} \frac{1}{2}{\penaltyC}{\condbrscale}\tpose \mathbf{I}\condbrscale  \text{~where~} \condZbasisR=\condXbasisR \boldsymbol{D}_{+}^{-1/2}
\end{align*}
and $\boldsymbol{D}_{+}^{1/2}$ is a generalized square root.  

Hence the conditional model (\ref{eqn:flexCond1}) can be written
\begin{align}
\link\{\condmeani_{ij}(\covxi_{ij})\}&=\condXbasisF\condbetaF+ \condZbasisR\condbrscale+ \covz_{ij}\tpose \re_{i}, \text{ ~~~ } \re_{i} \sim N(\mathbf{0},\boldsymbol{\Sigma})\label{eqn:flexCond2}
\end{align}
subject to a quadratic penalty $\frac{1}{2}{\penaltyC}{\condbrscale}\tpose \mathbf{I}\condbrscale$. We can now exploit the duality between a quadratic penalty and a Gaussian prior on $\condbr$; maximizing the penalized likelihood for model \ref{eqn:flexCond2} can be operationalized by maximizing the likelihood of a GLMM where $\condbrscale$ are treated as random effects with prior $N(\mathbf{0},{\penaltyC}^{-1}\mathbf{I})$.  \glen{[Phrasing this in a somewhat cagey way since I'm having trouble with one detail: it's not quite the same objective function, because with a GLMM you marginalize out the random effects.]}

We fit the equivalent GLMM via restricted maximum likelihood (REML) by first marginalizing out the fixed and random effect and then maximizing the REML criterion
\begin{align}
\lik_{REML}(\penaltyC,\covmat;\data)\ \propto \ \int\exp\{ \ell(\condbetaF,\condbrscale,\re)-\frac{1}{2} \penaltyC {\condbrscale}\tpose {\condbrscale} -\frac{1}{2} {\re}\tpose \covmat  \re \} d (\re,\condbrscale,\condbetaF ) \label{eqn:REML}
\end{align}
with respect to the variance components (which includes the smoothing parameter $\penaltyC$), where $\ell(\condbetaF,\condbrscale,\re)$ is the log conditional likelihood, a sum of contributions each of exponential family form.  In practice we use a Laplace approximation to (\ref{eqn:REML}):
\begin{align}
\lik_{REML,LA}(\penaltyC,\covmat;\data)\ \propto\ |\mathbf{L}^{-1}| \exp\{ \ell(\condbetaFest,\condbrscalepred,\repred)-\frac{1}{2}\penaltyC {\condbrscalepredtpose}   {\condbrscalepred} -\frac{1}{2} {\repred}\tpose \covmat \repred \}  \label{eqn:REMLlaplace}
\end{align}
where $\mathbf{L}$ is the Cholesky matrix of the Hessian of the integrand in (\ref{eqn:REML}), and $\condbetaFest$, $\condbrscalepred$, and $\repred$ are the respective modes. These modes depend on the values of the variance components, so one must iterate between maximizing  (\ref{eqn:REMLlaplace}) with respect to the variance components, and maximizing $\ell(\condbetaF,\condbrscale,\re)-\frac{1}{2} \penaltyC {\condbrscale}\tpose  {\condbrscale} -\frac{1}{2} {\re}\tpose \covmat  \re $ holding the current variance components fixed.  At convergence, this results in the REML estimates of $ \condbetaFest,\covmatest,\penaltyCest$ as well as predictions $\condbrscalepred$, and $\repred$ (which are posterior modes). This is conducted via the {\tt{TMB}} package. Then, one can easily compute fitted smooths: $\widehat{\smoothfunC}(\mathbf{X})=\condXbasisF\condbetaFest+ \condZbasisR\condbrscalepred$.  See REML in GLMM references: \cite{millar2011maximum,wood2011fast,liao2002type,bellio2011restricted,berger1999integrated}

While we prefer REML because of its reduced bias in estimating variance components---which in this case are necessary for fitting the second stage marginal model---we could alternatively maximize the usual marginal likelihood for a GLMM:
\begin{align}
\lik_{ML}(\condbetaF,\penaltyC,\covmat;\data)\ \propto \ \int\exp\{ \ell(\condbetaF,\condbrscale,\re)-\frac{1}{2} \penaltyC {\condbrscale}\tpose  {\condbrscale} -\frac{1}{2} {\re}\tpose \covmat  \re \} d (\re,\condbrscale ). \label{eqn:ML}
\end{align}
We again adopt a Laplace approximation to this:
\begin{align}
\lik_{ML,LA}(\condbetaF,\penaltyC,\covmat;\data)\ \propto\ |\mathbf{L}^{-1}| \exp\{ \ell(\condbetaF,\condbrscalepred,\repred)-\frac{1}{2}\penaltyC {\condbrscalepredtpose} {\condbrscalepred} -\frac{1}{2} {\repred}\tpose \covmat \repred \},  \label{eqn:MLlaplace}
\end{align}
this time iterating between updating with respect to $\condbetaF$, $\penaltyC$ and $\covmat$ by maximizing (\ref{eqn:MLlaplace}), and then maximizing the integrand in (\ref{eqn:ML}) with respect to $\condbrscalepred$ and $\repred$.

%\glen{[Does jointly minimizing w.r.t. $\condbetaFest$ and $\repred$ and  $\condbrscalepred$  really achieve the ML estimates? Typically  $\condbetaFest$ is estimated by marginalizing out the random effects, and random effect predictions can be computed post hoc]}

\subsection{Step 2: Compute the pseudo-outcomes (marginal means)}
\label{ss:step2}

By law of iterated expectation
\begin{align}
	\margmeani_{ij}(\covxi_{ij}) =\ \int \invlink\left\lbrace \smoothfunC(\covxi_{ij}) +\ \covz_{ij}\tpose \re_i \right\rbrace d\redist(\re_i; \covmat),  \label{eqn:inteq_flex2}
\end{align}
and we estimate  $\margmeanlinki_{ij}\equiv\link\left\lbrace \margmeani_{ij}(\covxi_{in_i})\right\rbrace$, by evaluating (\ref{eqn:inteq_flex2}) where we set  $\smoothfunC(\covxi_{ij})= \smoothfunCest(\covxi_{ij})$ and $\covmat=\covmatest$ from the fitted conditional model. Let $\margmeanlinkesti_{ij}(\covxi_{ij})$ denote the resulting estimator based on a Laplace approximation to (\ref{eqn:inteq_flex2}):
\begin{align}
	\margmeanlinkesti_{ij}(\covxi_{ij}) &=g\left[ (2\pi)^{d/2}~|\widehat{\mathbf{L}}^{-1}|~  \invlink\left\lbrace \smoothfunCest(\covxi_{ij}) +\ \covz_{ij}\tpose \repred_i \right\rbrace  ~f(\repred_i; \covmatest)    \right]  \label{eqn:laplace}
\end{align}
where  $d$ is the dimension of the integral, $\widehat{\mathbf{L}}$ is the Cholesky matrix of the Hessian of the log-integrand evaluated at mode of the integrand $\repred_i$, and $f(\repred_i; \covmatest)$ represents a multivariate Gaussian distribution with variance $\covmatest$ and evaluated at $\repred_i$. \glen{[This $\repred_i$ is different than our predictions/posterior modes above, right?] }

We note here that this need not be restricted to the observed exposures $\covx_{ij}$. Rather, we can estimate 	$\margmeanlinkesti_{ij}(\covxi_*)$ for any arbitrary covariate $\covxi_{*}$. Let $\margmeanlinkest$ be the resulting vector of estimates $\margmeanlinkesti_{ij}(\covxi_*)$ for an arbitrary grid of exposures $\covx_*$.

\subsection{Step 3: Fit the marginal model to the pseudo-outcomes}
\label{ss:step3}
Consider now the marginal model of interest:
 \begin{align}
	\margmeanlinki_{ij}(\covxi_{ij})\equiv\link\left(E[\datai_{ij}|\covxi_{ij}]\right)\ &=\ \smoothfunM(\covxi_{ij}), \label{eqn:flexMarg2}
\end{align}
For some basis  $\{\margbasisfun_q(x)\}_{q=1}^Q$, we express
$\smoothfunM(x)=\sum_{q=1}^Q \margbasisfun_q (x) \margbasiscoefi_q$ with a quadratic penalty $\penaltyM{\margbasiscoef}\tpose \margSmat \margbasiscoef/2$ where $\margbasiscoef=[\margbasiscoefi_1,\dots, \margbasiscoef_Q]^T$ is a vector of unknown coefficients, $\margSmat$ is a known $Q\times Q$ positive semi definite matrix determined by the basis and $\penaltyM$ is a smoothing parameter to be estimated.  Write $\smoothfunM(\mathbf{x})=\margXbasis \margbasiscoef$ where $\margbasiscoef$ is the induced model matrix, and as above:
\begin{align*}
\smoothfunM(\mathbf{x})&=\margXbasis \margbasiscoef \\
%&=\margXbasisF\margbetaF+ \margXbasisR\margbr \text{~~ where ~~} \margbr\sim N(\mathbf{0},[{\penaltyM}]^{-1}\mathbf{D'}_{+}^{-1}).
&=\margXbasisF\margbetaF+ \margXbasisR\margbr \text{~~ subject to ~~} {\penaltyM}{\margbr}\tpose [\mathbf{D}_{+}^{\texttt{M}} ]^{-1} \margbr.
\end{align*}
We exploit the duality between additive models and  linear mixed model representation. Treating $\penaltyM$ as a variance component in a linear mixed model, we first estimate $\penaltyM$ by REML as in \cite{wood2011fast}. Then, conditional on this estimate it is straightforward to obtain the usual (weighted) penalized least squares estimator
\begin{align}
\margbasiscoefest&={({\margXbasis}\tpose  \margXbasis+{\penaltyMest} \margSmat)}^{-1}\margXbasis  \margmeanlinkest.
\end{align}
 Then we can easily compute estimates of the smooth functions: $\widehat{\smoothfunM}(\mathbf{x})=\margXbasis \margbasiscoefest$.
%

%\weightmatest^{-1}

%
%If we could directly observe the $	\margmeanlinki_{ij}(\covxi_{ij})$ values, this would simply be an additive model. As such we treat $\margmeanlinkest$ as a vector of pseudo-outcomes, and fit the following additive model:
% \begin{align}
%\margmeanlinkest  &=\ \smoothfunM(\covx_*), \label{eqn:flexMargPseudo}
%\end{align}
%where $\text{Var}(\margmeanlinkest)=\boldsymbol{\Psi}$. 
%

\section{B: Standard Errors}
\label{s:appendixB}

\subsection{Step 1: Conditional Model}
For simplicity, let $\varcompC$ be the vector of all variance components in $\covmat$ as well as smoothing parameters $\penaltyC$ in the conditional model, and let $\varcompCest$ be the vector of corresponding estimates.

The derivative comes from  \cite{kristensen2015tmb}

 The variance correction term comes from \cite{kass1989approximate} and is based on the law of total expectation and the delta method (Taylor expansion)   % check out simon wood 2016 for argument about approximate bayesian inference

At the first step, we estimate the variance matrix of coefficients $[{\condbr}\tpose, {\condbetaF}\tpose]\tpose$ as in \cite{wood2016smoothing}. In particular, we must capture for uncertainty in the estimates of the variance components themselves in order to properly propagate uncertainty in Step 2.  \cite{kass1989approximate} proposed a corrected variance estimate that is equal to the usual (naive) variance matrix treating the variance/smoothing components as fixed, plus a correction term, which follows from the law of total variance and first order Taylor approximations. The large sample approximate variance of $[{\condbr}\tpose, {\condbetaF}\tpose]\tpose$, $\VarC$, is estimated by 
\begin{align*}
\VarCest&=\VarCestUncorr+ \left(\derivkass \right) \VarCvarcompest  \left(\derivkass \right)\tpose \\
\VarCestUncorr&= (\infoCest+\penaltyCest \condSmat)^{-1}\infoCest(\infoCest+\penaltyCest \condSmat)^{-1} \\
\derivkass&= -\left( \VarCestUncorr \right)^{-1} \HstC
\end{align*}
where $\VarCestUncorr$ is the naive variance estimator treating the variance components as fixed,  $\VarCvarcompest$ is the negative inverse Hessian of the \textit{marginal} log likelihood for the variance components (i.e. after integrating out all fixed and random effects), $\infoCest$ is the negative inverse Hessian of the conditional log likelihood of fixed and random effects alike (treating variance components as fixed).  The final line follows from \cite{kristensen2015tmb}, where $\HstC =\frac{\partial^2}{\partial\condbasiscoefest\partial \varcompCest}\log\mathcal{P}$ is a matrix of second derivatives of the log posterior. Alternatively, a large sample Bayesian approximation follows by replacing $\VarCestUncorr$ by $(\infoCest+\penaltyCest \condSmat)^{-1}$.

\glen{Need the entire covariance matrix for both fixed/random effects as well as the variance components. Right now we have the marginal covariance matrices of both. Suppose we }

\subsection{Step 2: Pseudo-outcomes}

Given the estimated joint covariance matrix for fixed, random and variance components, $\VarCestall$, from the conditional model obtained in Step 1, we apply the multivariate delta method to estimate the  covariance matrix for the pseudo outcomes, $\margmeanlinkest$:
\begin{align*}
\weightmatest&=\left(\mathbf{d}\right)^T \VarCestall \left(\mathbf{d}\right)
\end{align*}

\subsection{Step 3: Marginal Model}
Treating $\penaltyMest$ as fixed, we have that:
\begin{align}
\VarMUncorr&\equiv \text{Var}\left({({\margXbasis}\tpose  \margXbasis+{\penaltyMest} \margSmat)}^{-1}\margXbasis  \margmeanlinkest\right) \\
	&={({\margXbasis}\tpose  \margXbasis+{\penaltyMest} \margSmat)}^{-1}\margXbasis  \text{Var}\left(\margmeanlinkest\right) {\margXbasis}\tpose {({\margXbasis}\tpose  \margXbasis+{\penaltyMest} \margSmat)}^{-1} 
\end{align}
which we can estimate by
\begin{align}
	\VarMestUncorr&={({\margXbasis}\tpose  \margXbasis+{\penaltyMest} \margSmat)}^{-1}\margXbasis  \weightmatest {\margXbasis}\tpose {({\margXbasis}\tpose  \margXbasis+{\penaltyMest} \margSmat)}^{-1} 
\end{align}
where $\weightmatest$ is the estimated variance-covariance matrix of $\margmeanlinkest$ from Step 2. However this ignores uncertainty in the smoothing parameters, so again use a corrected variance estimate following \cite{kass1989approximate}:
\begin{align*}
	\VarMest&=\VarMestUncorr+ \left(\derivkassM \right) \VarMvarcompest  \left(\derivkassM \right)\tpose \\
	\derivkassM&= -\left( \VarMestUncorr \right)^{-1} \HstM
\end{align*}
where $\VarMvarcompest$ is the negative inverse Hessian of the \textit{marginal} log likelihood for the variance components (i.e. after integrating out all fixed and random effects),  and  $\HstM =\frac{\partial^2}{\partial\margbasiscoefest \partial \penaltyMest}\log\mathcal{P}$ is a matrix of second derivatives of the penalized log likelihood.
